# Supplementary material for: Quantum Entropic Effects in the Liquid Viscosities of Hydrogen, Deuterium, and Neon
Source: arXiv:2303.05570 source file (2023-03-09)
Supplement: Supplementary file 1 [file SI_quantumentropypaper.pdf]

# Supporting Information: Quantum Entropic Effects in the Liquid Viscosities of Hydrogen, Deuterium, and Neon

Ian H. Bell,<sup>1,\*</sup> Jacob W. Leachman,<sup>2</sup> Albert F. Rigosi,<sup>3</sup> and Heather M. Hill<sup>3</sup>

<sup>1</sup>*Applied Chemicals and Materials Division, National Institute of Standards and Technology, Boulder, CO 80305, USA*

<sup>2</sup>*Hydrogen Properties for Energy Research Laboratory,*

*School of Mechanical and Materials Engineering,*

*Washington State University, Pullman, WA 99163, USA*

<sup>3</sup>*Quantum Measurement Division, National Institute of Standards and Technology, Gaithersburg, MD, 20899, USA*

## CONTENTS

|                                                          |    |
|----------------------------------------------------------|----|
| I. Equations of State                                    | 2  |
| II. Ideal-gas Entropy of a Bose-Einstein gas             | 2  |
| A. Reichl method                                         | 2  |
| B. Virial correction from Hill                           | 6  |
| C. Virial correction from Hill with additional terms     | 6  |
| 1. Definitions                                           | 6  |
| 2. Goal 1 of 6                                           | 6  |
| 3. Goal 2 of 6                                           | 6  |
| 4. Goal 3 of 6                                           | 7  |
| 5. Goal 4 of 6                                           | 7  |
| 6. Goal 5 of 6                                           | 9  |
| 7. Goal 6 of 6                                           | 10 |
| III. Experimental Data                                   | 12 |
| IV. Classical simulations                                | 15 |
| A. Interaction potentials                                | 15 |
| 1. Pair potentials                                       | 15 |
| 2. Three-body potentials                                 | 15 |
| B. Computer simulation                                   | 16 |
| 1. Simulation details                                    | 16 |
| 2. Locating the triple point                             | 16 |
| 3. Computing the residual entropy                        | 16 |
| C. Neon data                                             | 17 |
| D. Hydrogen data                                         | 17 |
| V. Cryogen trends                                        | 18 |
| VI. Thermodynamic Models for Real Gas Quantum Correction | 18 |
| A. Boltzmann correction                                  | 18 |
| B. Deiters quantum correction                            | 18 |
| C. Hard sphere with quantum effects                      | 21 |
| VII. $s^+$ at triple point                               | 22 |
| A. Ideal-gas                                             | 22 |
| B. Liquid phase                                          | 22 |
| C. Walker model                                          | 23 |
| References                                               | 24 |

---

\* ian.bell@nist.gov; Corresponding author

## I. EQUATIONS OF STATE

The equations of state used in the reference EOS libraries of NIST REFPROP, CoolProp, and TREND are all of the Helmholtz energy formulation. This formulation gives the total Helmholtz energy  $a$  as the sum of a non-interacting ideal-gas part given by  $a^{\text{ig}}$  and an excess term accounting for interaction

$$a = a^{\text{ig}} + a^{\text{ex}}. \quad (1)$$

In the EOS literature and in chemical thermodynamics, the “excess” contribution is always denoted as the residual contribution, but for consistency with the physics literature, we will denote here the interaction contribution as the “excess” one.

The terms are non-dimensionalized by the product of  $k_{\text{B}}T$  where the  $a$  are per-particle Helmholtz energies. This yields the contributions  $\alpha = a/(k_{\text{B}}T)$ . The value of the excess entropy divided by  $k_{\text{B}}$  is thus given by

$$\frac{s^{\text{ex}}}{k_{\text{B}}} = -T \left( \frac{\partial \alpha^{\text{ex}}}{\partial T} \right)_{\rho} - \alpha^{\text{ex}}. \quad (2)$$

Other thermodynamic properties are obtained in a similar fashion. See for instance the appendix of Bell et al.[1] or Span[2].

The particular form of the EOS is entirely empirical, and the coefficients for each EOS should be taken from the corresponding reference.

## II. IDEAL-GAS ENTROPY OF A BOSE-EINSTEIN GAS

Being species that have a sum of (electrons + protons + neutrons) that is an even number, the most prevalent isotope of the noble gases,  $\text{D}_2$ , and  $\text{H}_2$  all follow Bose-Einstein statistics ( $^3\text{He}$  follows Fermi-Dirac statistics). For the species considered here:

- $^1_1\text{H}$ : 1 electron, 0 neutron, 1 proton (Bose-Einstein statistics)
- $^1_1\text{H}_2$ : 2 electrons, 0 neutron, 2 protons (Bose-Einstein statistics)
- $^2_1\text{D}$ : 1 electron, 1 neutron, 1 proton (Fermi-Dirac statistics)
- $^2_1\text{D}_2$ : 2 electrons, 2 neutrons, 2 protons (Bose-Einstein statistics)
- $^{20}_{10}\text{Ne}$ : 10 electrons, 10 neutrons, 10 protons (Bose-Einstein statistics)
- $^3_2\text{He}$ : 2 electrons, 1 neutrons, 2 protons (Fermi-Dirac statistics)
- $^4_2\text{He}$ : 2 electrons, 2 neutrons, 2 protons (Bose-Einstein statistics)

### A. Reichl method

In Eq. 6.87 of Reichl [3], the entropy  $S$  per volume  $V$  of a Bose-Einstein fluid is given in terms of the absolute activity (Reichl refers to this quantity as the fugacity)  $z = \exp(\mu/(k_{\text{B}}T))$  (for  $z$  less than 1):

$$\frac{S}{V} = k_{\text{B}} \left( \frac{5}{2} \frac{1}{\lambda_{\text{th}}^3} g_{5/2}(z) - \langle n \rangle \ln z \right) \quad (3)$$

in terms of the total number density of particles  $\langle n \rangle$  and the function  $g_{5/2}$  is

$$g_{5/2}(z) = \sum_{k=1}^{\infty} \frac{z^k}{k^{5/2}}. \quad (4)$$

And multiplying through by  $V/N$  (the reciprocal of the number density  $\rho_{\text{N}}$ ), one obtains

$$\frac{S}{Nk_{\text{B}}} = \frac{5}{2} \frac{V}{N\lambda_{\text{th}}^3} g_{5/2}(z) - \frac{V}{N} \langle n \rangle \ln z \quad (5)$$

In Eq. 6.74 of Reichl the total number density of particles  $\langle n \rangle$  in the ground- and elevated-energy states is defined by

$$\langle n \rangle = \frac{1}{V} \frac{z}{1-z} + \frac{1}{\lambda_{\text{th}}^3} g_{3/2}(z) \quad (6)$$

and in the limit of the system size being macroscopic ( $V$  going to  $\infty$ ),

$$\lim_{V \rightarrow \infty} \langle n \rangle = \frac{1}{\lambda_{\text{th}}^3} g_{3/2}(z) \quad (7)$$

we obtain

$$\frac{S}{Nk_B} = \frac{5}{2} \frac{V}{N\lambda_{\text{th}}^3} g_{5/2}(z) - \frac{V}{N} \frac{1}{\lambda_{\text{th}}^3} g_{3/2}(z) \ln z \quad (8)$$

After defining  $\rho_N = N/V = \langle n \rangle$ , the total entropy is obtained from

$$\frac{S}{Nk_B} = \frac{5}{2} \frac{g_{5/2}(z)}{\rho_N \lambda_{\text{th}}^3} - \frac{g_{3/2}(z) \ln z}{\rho_N \lambda_{\text{th}}^3} \quad (9)$$

From Eq. (7), the value of  $\frac{g_{3/2}(z)}{\rho_N \lambda_{\text{th}}^3}$  is 1, simplifying to

$$\frac{S}{Nk_B} = \frac{5}{2} \frac{g_{5/2}(z)}{\rho_N \lambda_{\text{th}}^3} - \ln z \quad (10)$$

The absolute activity  $z$  is obtained by iteratively solving Eq. (7) for the given value of  $\rho_N \lambda_{\text{th}}^3$  in which

$$g_{3/2}(z) = \sum_{k=1}^{\infty} \frac{z^k}{k^{3/2}}. \quad (11)$$

The function  $g_{3/2}(z)$  is a monotonic function of  $z$  so inverting the function to solve for  $z$  (in  $(0,1)$ ) given a value of  $\rho_N \lambda_{\text{th}}^3$  can be achieved with a bounded rootfinding method. Thus the equation for the entropy of a Bose-Einstein fluid, subject to the assumptions:

- absolute activity  $z$  is less than 1
- $N$  is very large, and so is  $V$ , but their ratio (the number density) is finite

is a function of only the combined term  $\rho_N \lambda_{\text{th}}^3$ . The shape of this curve is shown in Fig. 1. The contribution from the quantum terms is approximately  $0.09k_B$  at  $\mathcal{L} = 1$ .

This result should be compared with the Sackur-Tetrode result for a classical monatomic ideal gas:

$$\frac{S_{\text{Sackur-Tetrode}}}{Nk_B} = \frac{5}{2} - \ln(\rho_N \lambda_{\text{th}}^3) \quad (12)$$

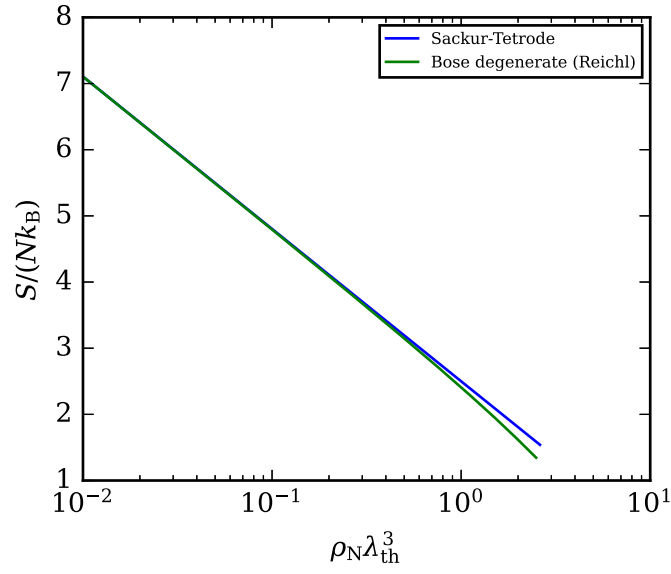

FIG. 1. Entropy of the ideal-gas Bose-Einstein fluid as a function of  $\rho_N \lambda_{\text{th}}^3$

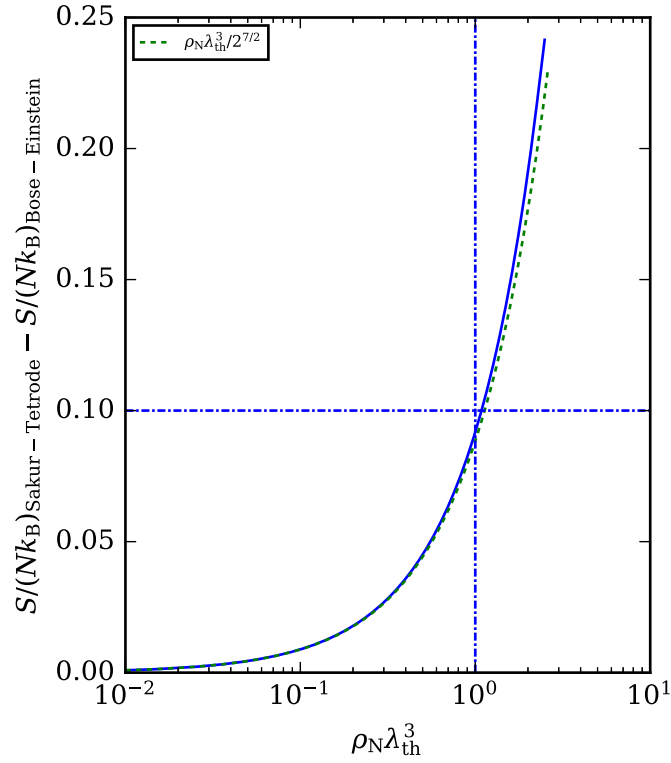

FIG. 2. Difference of the entropy of the ideal-gas Bose-Einstein fluid from that of the Sackur-Tetrode equation as a function of  $\rho_N \lambda_{\text{th}}^3$  and the first term in the virial expansion

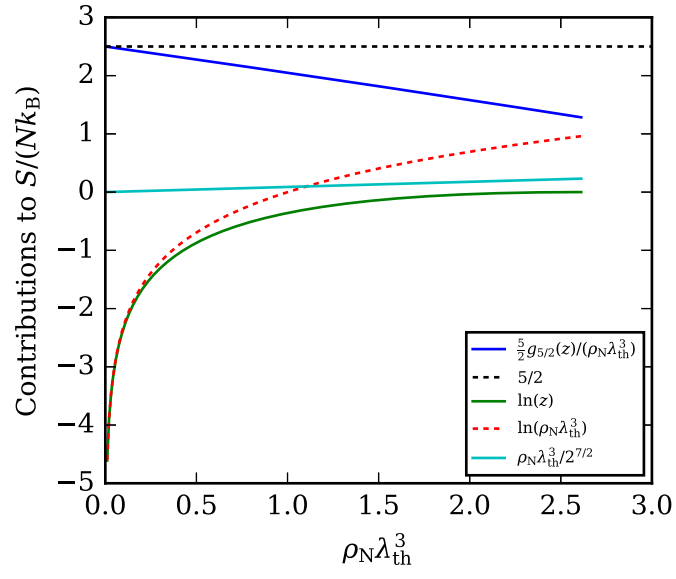

FIG. 3. Contributions to the entropy of the ideal-gas Bose-Einstein fluid as a function of  $\rho_N \lambda_{th}^3$ . The dashed curves correspond to the contributions present in the Sackur-Tetrode equation.

## B. Virial correction from Hill

The monograph of Hill[4] derives the contributions for the Bose-Einstein fluid, up to the first term in the virial expansion. This yields the term for the reduced chemical potential of (from Hill[4], Eq. 22-29)

$$\ln z = \frac{\mu}{k_B T} = \ln(\mathcal{L}^3) - \frac{\mathcal{L}^3}{2^{7/2}} + \dots \quad (13)$$

and the entropy is then obtained from Eq. 22-41 in Hill[4]:

$$\frac{S}{N k_B} = \frac{5}{2} - \ln(\mathcal{L}^3) - \frac{\mathcal{L}^3}{2^{7/2}} + \dots \quad (14)$$

The right-most term is plotted in Fig. 2 to highlight that most of the difference is coming from this first term. The next section derives the next few terms in the expansion.

A similar correction term was provided in Eq. 55.14 in Landau and Lifshitz[5]

## C. Virial correction from Hill with additional terms

### 1. Definitions

Starting with the textbook definition from Eq. 22-35 of Hill[4]:

$$\frac{p}{k_B T} = \sum_{j \geq 1} \frac{(\mp 1)^{j-1} \lambda_{\text{th}}^{3(j-1)}}{j^{5/2}} z^j = \sum_{j \geq 1} b_j(T) z^j \quad (15)$$

where the upper sign applies to Fermi-Dirac particles, and the lower to Bose-Einstein particles. The de Broglie wavelength is defined by

$$\lambda_{\text{th}} \equiv \frac{h}{\sqrt{2\pi m \frac{k_B}{den} T}} \quad (16)$$

The goals will be to:

1. Get  $\frac{p}{k_B T}$  in terms of a polynomial of order  $z^{10}$
2. Get  $\rho$  in terms of that same polynomial variable of order  $z^{10}$
3. Transform  $z$  into a tenth-order polynomial in  $\rho$
4. Equate all lower-case coefficients (in order of higher ranking powers of  $\rho$ ) to express  $\frac{p}{k_B T}$  as a function of  $\rho$
5. Get  $\frac{p}{k_B T}$  as a function of  $\rho$  and  $b_j$  and solve for all virial coefficients up to  $B_{10}$
6. Expand  $\frac{S}{Nk}$  in the new terms

### 2. Goal 1 of 6

$$\frac{p}{k_B T} = b_1 z + b_2 z^2 + b_3 z^3 + b_4 z^4 + b_5 z^5 + b_6 z^6 + b_7 z^7 + b_8 z^8 + b_9 z^9 + b_{10} z^{10} \quad (17)$$

Note that  $b_1 = 1$  due to Eq. (15).

### 3. Goal 2 of 6

In order to link  $\rho$  to  $z$ , we use the partial differential equation in Eq. 15-9 of Hill[4]. This linking will be vital for the algebraic analysis done in Goal 4. The series expansion reads

$$\rho = z \left( \frac{\partial \frac{p}{k_B T}}{\partial z} \right)_T = z + 2b_2 z^2 + 3b_3 z^3 + 4b_4 z^4 + 5b_5 z^5 + 6b_6 z^6 + 7b_7 z^7 + 8b_8 z^8 + 9b_9 z^9 + 10b_{10} z^{10} \quad (18)$$

#### 4. Goal 3 of 6

Define  $z$  in terms of a polynomial in  $\rho$  with new coefficients  $a_i$ :

$$z = a_1\rho + a_2\rho^2 + a_3\rho^3 + a_4\rho^4 + a_5\rho^5 + a_6\rho^6 + a_7\rho^7 + a_8\rho^8 + a_9\rho^9 + a_{10}\rho^{10} \quad (19)$$

(Note that it will be determined that  $a_1 = 1$ ). At this point, one may substitute this expression for all orders of  $z$  in Eq. (18) to get a fully expanded formula for  $\rho$  that now contains coefficients  $a_i$  and  $b_j$ .

#### 5. Goal 4 of 6

This lengthy expansion of Eq. (18) should now be compared in terms of the coefficients of each order of magnitude of  $\rho$ . For instance, the left side of the equation contains a single  $\rho$  with coefficient 1, which one may now equate with the coefficients of  $\rho$  on the right side of the equation. Since it's just  $a_1$ , then it follows that  $a_1 = 1$ . Every other order of magnitude of  $\rho$  on the left side of the expanded Eq. (18) has a coefficient of 0, meaning that all coefficients on the right side, per order of magnitude of  $\rho$ , must also equate to 0:

$$\mathcal{O}(\rho^2) : 0 = a_2 + 2b_2 \quad (20)$$

$$\mathcal{O}(\rho^3) : 0 = a_3 + 4a_2b_2 + 3b_3 \quad (21)$$

$$\mathcal{O}(\rho^4) : 0 = a_4 + 2a_2^2b_2 + 4a_3b_2 + 9a_2b_3 + 4b_4 \quad (22)$$

$$\mathcal{O}(\rho^5) : 0 = a_5 + 4a_2a_3b_2 + 4a_4b_2 + 9a_2^2b_3 + 9a_3b_3 + 16a_2b_4 + 5b_5 \quad (23)$$

$$\begin{aligned} \mathcal{O}(\rho^6) : 0 = a_6 + 2a_3^2b_2 + 4a_2a_4b_2 + 4a_5b_2 + 3a_2^3b_3 + 18a_2a_3b_3 + 9a_4b_3 + \\ \dots \\ + 24a_2^2b_4 + b_4 + 16a_3b_4 + 25a_2b_5 + 6b_6 \end{aligned} \quad (24)$$

$$\begin{aligned} \mathcal{O}(\rho^7) : 0 = a_7 + 4a_3a_4b_2 + 4a_2a_5b_2 + 4a_6b_2 + 9a_3^2b_3 + 9a_2^2a_3b_3 + 18a_2a_4b_3 + \\ \dots \\ + 9a_5b_3 + 16a_2^3b_4 + 48a_2a_3b_4 + 16a_4b_4 + 50a_2^2b_5 + 25a_3b_5 + 36a_2b_6 + 7b_7 \end{aligned} \quad (25)$$

$$\begin{aligned} \mathcal{O}(\rho^8) : 0 = a_8 + 2a_4^2b_2 + 4a_3a_5b_2 + 4a_2a_6b_2 + 4a_7b_2 + 9a_2a_3^2b_3 + 9a_2^2a_4b_3 + 18a_3a_4b_3 + 18a_2a_5b_3 + \\ \dots \\ + 9a_6b_3 + 4a_2^4b_4 + 24a_3^2b_4 + 48a_2^2a_3b_4 + 48a_2a_4b_4 + 16a_5b_4 + 50a_2^3b_5 + 100a_2a_3b_5 + \\ \dots \\ + 25a_4b_5 + 90a_2^2b_6 + 36a_3b_6 + 49a_2b_7 + 8b_8 \end{aligned} \quad (26)$$

$$\begin{aligned}
\mathcal{O}(\rho^9) : 0 = & a_9 + 4a_4a_5b_2 + 4a_3a_6b_2 + 4a_2a_7b_2 + 4a_8b_2 + 3a_3^3b_3 + 9a_4^2b_3 + 18a_2a_3a_4b_3 + \\
& \dots \\
& + 9a_2^2a_5b_3 + 18a_3a_5b_3 + 18a_2a_6b_3 + 9a_7b_3 + 48a_2a_3^2b_4 + 16a_2^3a_3b_4 + 48a_2^2a_4b_4 + 48a_3a_4b_4 + \\
& \dots \\
& + 48a_2a_5b_4 + 16a_6b_4 + 25a_2^4b_5 + 50a_3^2b_5 + 150a_2^2a_3b_5 + 100a_2a_4b_5 + 25a_5b_5 + \\
& \dots \\
& + 120a_2^3b_6 + 180a_2a_3b_6 + 36a_4b_6 + 147a_2^2b_7 + 49a_3b_7 + 64a_2b_8 + 9b_9 \quad (27)
\end{aligned}$$

$$\begin{aligned}
\mathcal{O}(\rho^{10}) : 0 = & a_{10} + 10b_{10} + 2a_5^2b_2 + 4a_4a_6b_2 + 4a_3a_7b_2 + 4a_2a_8b_2 + 4a_9b_2 + 9a_2a_4^2b_3 + \\
& \dots \\
& + 9a_3^2a_4b_3 + 18a_2a_3a_5b_3 + 18a_4a_5b_3 + 9a_2^2a_6b_3 + 18a_3a_6b_3 + 18a_2a_7b_3 + 9a_8b_3 + 16a_3^3b_4 + \\
& \dots \\
& + 24a_2^2a_3^2b_4 + 24a_4^2b_4 + 16a_2^3a_4b_4 + 96a_2a_3a_4b_4 + 48a_2^2a_5b_4 + 48a_3a_5b_4 + 48a_2a_6b_4 + 16a_7b_4 + \\
& \dots \\
& + 5a_2^5b_5 + 150a_2a_3^2b_5 + 100a_2^3a_3b_5 + 150a_2^2a_4b_5 + 100a_3a_4b_5 + 100a_2a_5b_5 + 25a_6b_5 + 90a_2^4b_6 + \\
& \dots \\
& + 90a_3^2b_6 + 360a_2^2a_3b_6 + 180a_2a_4b_6 + 36a_5b_6 + 245a_2^3b_7 + 294a_2a_3b_7 + \\
& \dots \\
& + 49a_4b_7 + 224a_2^2b_8 + 64a_3b_8 + 81a_2b_9 \quad (28)
\end{aligned}$$

This lengthy system of equations is solvable for all  $a_i$  coefficients in terms of  $b_j$  coefficients. The final results are:

$$a_1 = b_1 = 1 \quad (29)$$

$$a_2 = -2b_2 \quad (30)$$

$$a_3 = 8b_2^2 - 3b_3 \quad (31)$$

$$a_4 = -40b_2^3 + 30b_2b_3 - 4b_4 \quad (32)$$

$$a_5 = 224b_2^4 - 252b_2^2b_3 + 27b_3^2 + 48b_2b_4 - 5b_5 \quad (33)$$

$$a_6 = -1344b_2^5 + 2016b_2^3b_3 - 504b_2b_3^2 - 448b_2^2b_4 + 84b_3b_4 + 70b_2b_5 - 6b_6 \quad (34)$$

$$\begin{aligned}
a_7 = & 8448b_2^6 - 15840b_2^4b_3 + 6480b_2^2b_3^2 - 324b_3^3 + 3840b_2^3b_4 - 1728b_2b_3b_4 + 64b_4^2 - 720b_2^2b_5 + \\
& \dots \\
& + 120b_3b_5 + 96b_2b_6 - 7b_7 \quad (35)
\end{aligned}$$

$$\begin{aligned}
a_8 = & -54912b_2^7 + 123552b_2^5b_3 - 71280b_2^3b_3^2 + 8910b_2b_3^3 - 31680b_2^4b_4 + 23760b_2^2b_3b_4 \\
& \dots \\
& - 1620b_3^2b_4 - 1440b_2b_4^2 + 6600b_2^3b_5 - 2700b_2b_3b_5 + 180b_4b_5 - 1080b_2^2b_6 + \\
& \dots \\
& + 162b_3b_6 + 126b_2b_7 - 8b_8 \quad (36)
\end{aligned}$$

$$\begin{aligned}
a_9 = & 366080b_2^8 - 960960b_2^6b_3 + 720720b_2^4b_3^2 - 154440b_2^2b_3^3 + 4455b_3^4 + 256256b_2^5b_4 \\
& \dots \\
& - 274560b_2^3b_3b_4 + 47520b_2b_3^2b_4 + 21120b_2^2b_4^2 - 2640b_3b_4^2 - 57200b_2^4b_5 + \\
& \dots \\
& + 39600b_2^2b_3b_5 - 2475b_3^2b_5 - 4400b_2b_4b_5 + 125b_5^2 + 10560b_2^3b_6 - 3960b_2b_3b_6 + \\
& \dots \\
& + 240b_4b_6 - 1540b_2^2b_7 + 210b_3b_7 + 160b_2b_8 - 9b_9 \quad (37)
\end{aligned}$$

$$\begin{aligned}
a_{10} = & -10b_{10} - 2489344b_2^9 + 7468032b_2^7b_3 - 6918912b_2^5b_3^2 + 2162160b_2^3b_3^3 - 162162b_2b_3^4 \\
& \dots \\
& - 2050048b_2^6b_4 + 2882880b_2^4b_3b_4 - 864864b_2^2b_3^2b_4 + 30888b_3^3b_4 \\
& \dots \\
& - 256256b_2^3b_4^2 + 82368b_2b_3b_4^2 - 1408b_4^3 + 480480b_2^5b_5 - 480480b_2^3b_3b_5 + 77220b_2b_3^2b_5 + \\
& \dots \\
& + 68640b_2^2b_4b_5 - 7920b_3b_4b_5 - 3300b_2b_5^2 - 96096b_2^4b_6 + 61776b_2^2b_3b_6 - 3564b_3^2b_6 \\
& \dots \\
& - 6336b_2b_4b_6 + 330b_5b_6 + 16016b_2^3b_7 - 5544b_2b_3b_7 + 308b_4b_7 - 2112b_2^2b_8 + 264b_3b_8 + 198b_2b_9 \quad (38)
\end{aligned}$$

## 6. Goal 5 of 6

With  $z$  now a function of  $\rho$  and  $b_j$ , one can now obtain  $\frac{p}{k_B T}$  (Eq. (17)) as a function of  $\rho$  and  $b_j$ . If one substitutes every  $z$  as defined in Eq. (19), along with substituting all  $a_i$  coefficients in terms of  $b_j$ , all virial coefficients up to  $B_{10}$  can be determined from the following form:

$$\frac{p}{k_B T} = \rho + [f(b_i)] \rho^2 + [\dots \text{every order in } \rho \dots] + [g(b_i)] \rho^{10} \quad (39)$$

In this expression,  $B_2 = [f(b_i)]$  and  $B_{10} = [g(b_i)]$  since they are the coefficients of their respective order of  $\rho$ . For the sake of simplicity, this analysis is first done for Fermi-Dirac particles (selecting the top sign,  $-1$ , in Eq. (15)).

$$B_1 = 1 \quad (40)$$

$$B_2 = \frac{\lambda_{\text{th}}^3}{2^{5/2}} \quad (41)$$

$$B_3 = \frac{\lambda_{\text{th}}^6}{8} - \frac{2\lambda_{\text{th}}^6}{9\sqrt{3}} \quad (42)$$

$$B_4 = -\frac{\lambda_{\text{th}}^9}{2\sqrt{6}} + \frac{5\lambda_{\text{th}}^9}{32\sqrt{2}} + \frac{3\lambda_{\text{th}}^9}{32} \quad (43)$$

$$B_5 = -\frac{4\lambda_{\text{th}}^{12}}{25\sqrt{5}} + \frac{1}{8}\sqrt{3}\lambda_{\text{th}}^{12} - \frac{7\lambda_{\text{th}}^{12}}{8\sqrt{3}} + \frac{\lambda_{\text{th}}^{12}}{4\sqrt{2}} + \frac{317\lambda_{\text{th}}^{12}}{1728} \quad (44)$$

$$B_6 = -\frac{29\lambda_{\text{th}}^{15}}{50\sqrt{10}} - \frac{19\lambda_{\text{th}}^{15}}{12\sqrt{6}} - \frac{5\lambda_{\text{th}}^{15}}{24\sqrt{3}} - \frac{4}{81}\sqrt{2}\lambda_{\text{th}}^{15} + \frac{6085\lambda_{\text{th}}^{15}}{10368\sqrt{2}} + \frac{1}{4}\sqrt{\frac{3}{2}}\lambda_{\text{th}}^{15} + \frac{1}{25}\sqrt{\frac{2}{5}}\lambda_{\text{th}}^{15} + \frac{35\lambda_{\text{th}}^{15}}{128} \quad (45)$$

$$B_7 = \frac{2\lambda_{\text{th}}^{18}}{5\sqrt{15}} - \frac{6\lambda_{\text{th}}^{18}}{49\sqrt{7}} + \frac{\lambda_{\text{th}}^{18}}{2\sqrt{6}} - \frac{3\lambda_{\text{th}}^{18}}{5\sqrt{5}} - \frac{1019\lambda_{\text{th}}^{18}}{1296\sqrt{3}} + \frac{9\lambda_{\text{th}}^{18}}{16\sqrt{2}} - \frac{1}{2}\sqrt{\frac{3}{2}}\lambda_{\text{th}}^{18} + \frac{173\lambda_{\text{th}}^{18}}{256} \quad (46)$$

$$B_8 = -\frac{\lambda_{\text{th}}^{21}}{9\sqrt{30}} - \frac{\lambda_{\text{th}}^{21}}{2\sqrt{14}} - \frac{21\lambda_{\text{th}}^{21}}{16\sqrt{10}} + \frac{3559\lambda_{\text{th}}^{21}}{5184\sqrt{6}} - \frac{7\lambda_{\text{th}}^{21}}{40\sqrt{5}} - \frac{35}{64}\sqrt{3}\lambda_{\text{th}}^{21} - \frac{7}{81}\sqrt{2}\lambda_{\text{th}}^{21} + \dots + \frac{313573\lambda_{\text{th}}^{21}}{165888\sqrt{2}} - \frac{107}{128}\sqrt{\frac{3}{2}}\lambda_{\text{th}}^{21} - \frac{1}{25}\sqrt{\frac{6}{5}}\lambda_{\text{th}}^{21} + \frac{1}{81}\sqrt{\frac{2}{3}}\lambda_{\text{th}}^{21} + \frac{9}{10}\sqrt{\frac{3}{10}}\lambda_{\text{th}}^{21} - \frac{28}{225}\sqrt{\frac{2}{15}}\lambda_{\text{th}}^{21} + \frac{4361\lambda_{\text{th}}^{21}}{6144} \quad (47)$$

$$B_9 = \frac{8\lambda_{\text{th}}^{24}}{21\sqrt{21}} + \frac{3259\lambda_{\text{th}}^{24}}{600\sqrt{15}} - \frac{\lambda_{\text{th}}^{24}}{\sqrt{10}} - \frac{5\lambda_{\text{th}}^{24}}{7\sqrt{7}} - \frac{1163\lambda_{\text{th}}^{24}}{192\sqrt{6}} - \frac{913\sqrt{5}\lambda_{\text{th}}^{24}}{1728} + \frac{559\lambda_{\text{th}}^{24}}{576\sqrt{5}} + \frac{103}{512}\sqrt{3}\lambda_{\text{th}}^{24} \dots - \frac{130381\lambda_{\text{th}}^{24}}{41472\sqrt{3}} - \frac{2}{81}\sqrt{2}\lambda_{\text{th}}^{24} + \frac{22655\lambda_{\text{th}}^{24}}{10368\sqrt{2}} - \frac{1}{8}\sqrt{\frac{5}{3}}\lambda_{\text{th}}^{24} + \frac{35}{64}\sqrt{\frac{3}{2}}\lambda_{\text{th}}^{24} - \frac{19}{50}\sqrt{\frac{3}{5}}\lambda_{\text{th}}^{24} + \frac{2310418933\lambda_{\text{th}}^{24}}{1119744000} \quad (48)$$

$$B_{10} = -\frac{103\lambda_{\text{th}}^{27}}{294\sqrt{42}} + \frac{5473\lambda_{\text{th}}^{27}}{360\sqrt{30}} - \frac{99\lambda_{\text{th}}^{27}}{56\sqrt{14}} - \frac{4273\lambda_{\text{th}}^{27}}{600\sqrt{10}} - \frac{9\lambda_{\text{th}}^{27}}{56\sqrt{7}} - \frac{2073419\lambda_{\text{th}}^{27}}{248832\sqrt{6}} - \frac{297\lambda_{\text{th}}^{27}}{160\sqrt{5}} + \dots + \frac{71}{512}\sqrt{3}\lambda_{\text{th}}^{27} - \frac{3497\lambda_{\text{th}}^{27}}{576\sqrt{3}} + \frac{1129\sqrt{\frac{5}{2}}\lambda_{\text{th}}^{27}}{3456} - \frac{1666\sqrt{2}\lambda_{\text{th}}^{27}}{151875} + \frac{6183592549\lambda_{\text{th}}^{27}}{1244160000\sqrt{2}} + \dots + \frac{183\sqrt{\frac{3}{2}}\lambda_{\text{th}}^{27}}{1024} - \frac{2}{49}\sqrt{\frac{6}{7}}\lambda_{\text{th}}^{27} + \frac{7}{243}\sqrt{\frac{2}{3}}\lambda_{\text{th}}^{27} + \frac{11}{40}\sqrt{\frac{3}{5}}\lambda_{\text{th}}^{27} + \frac{38}{135}\sqrt{\frac{2}{5}}\lambda_{\text{th}}^{27} \dots - \frac{1}{5}\sqrt{\frac{3}{10}}\lambda_{\text{th}}^{27} - \frac{94}{45}\sqrt{\frac{2}{15}}\lambda_{\text{th}}^{27} + \frac{31}{21}\sqrt{\frac{2}{21}}\lambda_{\text{th}}^{27} + \frac{27577\lambda_{\text{th}}^{27}}{8192} \quad (49)$$

Note that these virial coefficients apply to Fermi-Dirac (F-D) cases only. For the Bose-Einstein cases (B-E), the results are similar and can be obtained from:

$$B_{1,3,5,7,9}^{\text{F-D}} = B_{1,3,5,7,9}^{\text{B-E}} \quad (50)$$

$$B_{2,4,6,8,10}^{\text{F-D}} = -B_{2,4,6,8,10}^{\text{B-E}} \quad (51)$$

## 7. Goal 6 of 6

With the virial coefficients determined, one must expand textbook equation (Eq. 22-37 from Hill[4]):

$$\frac{S}{\overline{N}k} = \frac{5}{2} - \ln(\rho\lambda_{\text{th}}^3) + \sum_{k \geq 1} \left( \frac{5}{2} - \frac{k+1}{k} \right) B_{k+1} \rho^k \quad (52)$$

which yields

$$\begin{aligned} \frac{S}{\overline{N}k} = \frac{5}{2} - \ln(\rho\lambda_{\text{th}}^3) + \frac{B_2}{2} \rho + B_3 \rho^2 + \left( \frac{5}{2} - \frac{4}{3} \right) B_4 \rho^3 + \left( \frac{5}{2} - \frac{5}{4} \right) B_5 \rho^4 + \left( \frac{5}{2} - \frac{6}{5} \right) B_6 \rho^5 \\ + \left( \frac{5}{2} - \frac{7}{6} \right) B_7 \rho^6 + \left( \frac{5}{2} - \frac{8}{7} \right) B_8 \rho^7 + \left( \frac{5}{2} - \frac{9}{8} \right) B_9 \rho^8 + \left( \frac{5}{2} - \frac{10}{9} \right) B_{10} \rho^9 \quad (53) \end{aligned}$$

As before, these results apply to F-D cases only, so suitable sign changes must be made for B-E cases (see Eqs. (50) to (51)).

### III. EXPERIMENTAL DATA

The selected datasets are listed in Table I. In some cases, in order to agree with the existing work [6, 7], some datapoints were removed that were deemed to be unreliable. Some additional datasets for normal hydrogen at high temperature and/or low density were not included.

TABLE I. The experimental datasets considered in this study. The column FLD refers to the identifier used in NIST REFPROP for the fluid.

| FLD      | author                          | $N_{\text{pts}}$ | $T_{\text{range}} / \text{K}$ |
|----------|---------------------------------|------------------|-------------------------------|
| D2       | van Itterbeek and van Paemel[8] | 20               | 18.74 - 23.65                 |
| HYDROGEN | Johns[9]                        | 42               | 14.2861 - 20.7035             |
| HYDROGEN | Kuss[10]                        | 27               | 298.1352 - 348.123            |
| HYDROGEN | Michels et al.[11]              | 95               | 298.1352 - 398.1281           |
| HYDROGEN | Diller[12]                      | 13               | 13.9952 - 25.9983             |
| HYDROGEN | Tsederberg et al.[13]           | 28               | 288.64 - 990.3516             |
| HYDROGEN | Rudenko and Slyusar[14]         | 52               | 150.014 - 299.9843            |
| HYDROGEN | Guevara et al.[15]              | 24               | 282.9933 - 2130.2947          |
| HYDROGEN | Golubiev[16]                    | 58               | 288.1463 - 523.1102           |
| HYDROGEN | Nabizadeh and Mayinger[17]      | 76               | 295.55 - 399.15               |
| NEON     | Forster[18]                     | 9                | 25.09 - 44.13                 |
| NEON     | Slyusar et al.[19]              | 18               | 24.7 - 44.4                   |
| PARAHYD  | Diller[12]                      | 328              | 14.0 - 100.0                  |

The location of the data points for parahydrogen and normal hydrogen are shown in Fig. 4 and Fig. 5. The data for parahydrogen cover much of the liquid phase, while the data for hydrogen cover only the saturated liquid state, as well as measurements at temperatures well above the critical point.

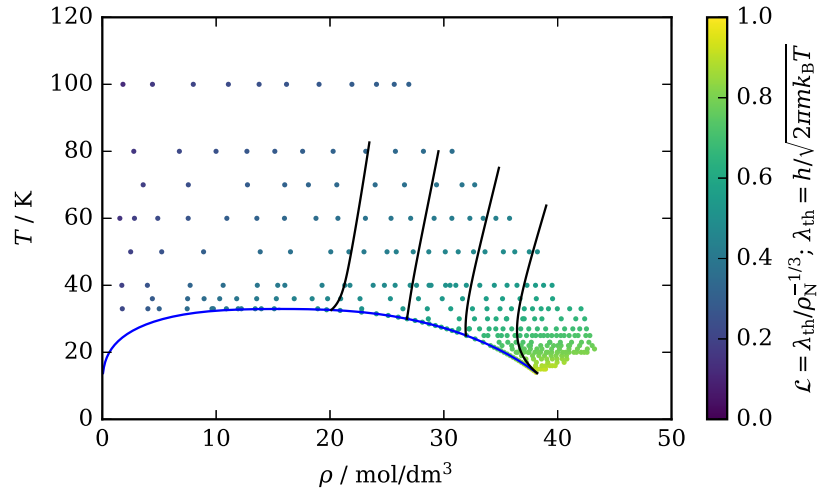

FIG. 4. Parahydrogen data points and curves of constant  $s^+$

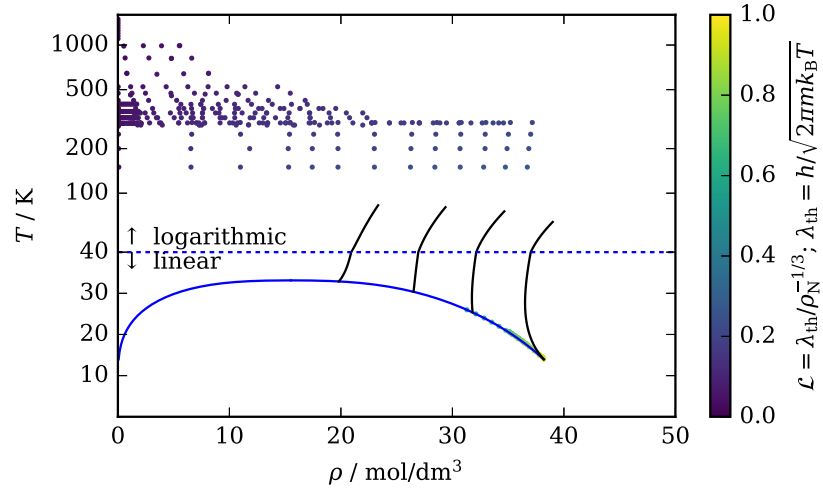

FIG. 5. Normal hydrogen data points and some curves of constant  $s^+$

In order to understand the impacts of the quantum effects, Fig. 6 and Fig. 7 show the values of reduced density (reduced by the critical point density) and reduced  $s^+$  (reduced by the critical point value of  $s^+$ ) along the vapor-liquid coexistence for both phases, with the saturated liquid as a solid curve and the saturated vapor as a dashed curve.

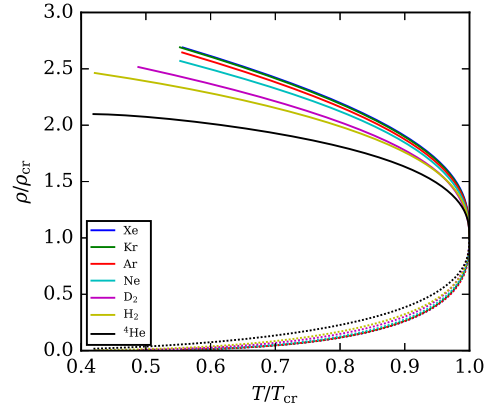

FIG. 6. Saturated liquid and vapor densities for cryogenes as a function of reduced temperature.

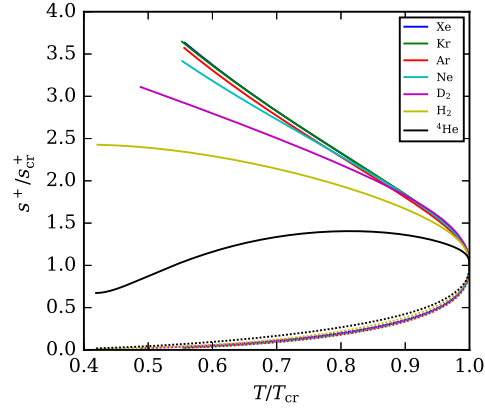

FIG. 7. Saturated liquid and vapor values of  $s^+$  for cryogenes.

## IV. CLASSICAL SIMULATIONS

### A. Interaction potentials

The interaction potentials used for this work are *ab initio* potentials, i.e., function obtained by computing the interaction energies of molecules by quantum mechanical methods without making use of experimental data—which would be difficult to obtain for hypothetical compounds.

#### 1. Pair potentials

The pair potentials of hydrogen and neon were represented by SAAP functions (simplified *ab initio* atomic potential) [20],

$$u_2(r) = \frac{\frac{a_0}{r} \exp(a_1 r) + a_2 \exp(a_3 r) + a_4}{1 + a_5 r^6}, \quad (54)$$

where the  $a_i$  are substance-specific parameters. For neon the  $a_i$  were fitted to the interaction energy data of Hellmann *et al.* [21]. For hydrogen the pair potential of Patkowski *et al.* [22] was used. As hydrogen is a molecule, its pair potential is angle-dependent. Only the isotropic term of the pair potential was used, i.e., it was assumed that the hydrogen molecule can be modeled as a sphere. The values of the pair potential parameters are listed in Table II.

#### 2. Three-body potentials

Of the many-body interaction potentials only the triple-dipole dispersion potential of Axilrod and Teller [23] and of Mutō [24] was considered (ATM),

$$u_3(r_{ij}, r_{jk}, r_{ik}) = \nu_{\text{ATM}} \frac{1 + 3 \cos \theta_i \cos \theta_j \cos \theta_k}{(r_{ij} r_{jk} r_{ik})^3}. \quad (55)$$

The  $\theta_i$  denote the inner angles of the triangle formed by the particles  $i$ ,  $j$ , and  $k$ .

The ATM potential can become negative and, at small distances, possibly outweigh the SAAP potential. A hard spherical core of diameter  $d_{\text{hs}}$  was therefore introduced as a protection against simulation artifacts. The ATM parameters are listed in Table II.

TABLE II. Dimensionless parameters of the SAAP pair potential Eq. (54) and the parameter of the ATM three-body potential used in this work ( $\epsilon$ : depth of the pair potential,  $\sigma$ : collision diameter ( $u(\sigma) = 0$ )).

[25]

|                                    | H <sub>2</sub>               | Ne                            |
|------------------------------------|------------------------------|-------------------------------|
| $(\epsilon/k_B)/K$                 | $3.624846199 \times 10^{+1}$ | $4.236165080 \times 10^{+1}$  |
| $\sigma/\text{\AA}$                | $3.044893462 \times 10^{+0}$ | $2.759124561 \times 10^{+0}$  |
| $a_0/(\sigma\epsilon/k_B)$         | $1.109296 \times 10^{+4}$    | $2.117818544 \times 10^{+5}$  |
| $a_1\sigma$                        | $-7.670023 \times 10^{+0}$   | $-1.089769496 \times 10^{+1}$ |
| $a_2/(\epsilon/k_B)$               | $-1.208954 \times 10^{+1}$   | $-2.094225988 \times 10^{+1}$ |
| $a_3\sigma$                        | $-1.689862 \times 10^{+0}$   | $-2.317079421 \times 10^{+0}$ |
| $a_4/(\epsilon/k_B)$               | $-2.944991 \times 10^{+0}$   | $-1.854049559 \times 10^{+0}$ |
| $a_5\sigma^6$                      | $9.832063 \times 10^{-1}$    | $7.454617542 \times 10^{-1}$  |
| $\nu_{\text{ATM}}/(\text{J cm}^9)$ | $6.82038 \times 10^{-91}$    | $1.7048 \times 10^{-91}$      |
| $d_{\text{hs}}/\text{\AA}$         | 1.80                         | 1.60                          |

## B. Computer simulation

### 1. Simulation details

The computer simulations required for this work were thermodynamic Monte Carlo simulations ( $NpT$  or  $NVT$  ensemble), executed with the program `mc++` [26].

The number of particles,  $N$ , was usually 864, with a spherical cut-off distance  $r_{\text{co}} = 4.5\sigma$ . For some simulations  $N = 1000$ ,  $r_{\text{co}} = 5.5$  was used.

The simulation box was cubic, with periodic boundary conditions (the fast version according to Ref. 27), and the common tail corrections for the pair potential cut-off were used.

As the contribution of the ATM term does not depend strongly on the configuration, the three-body energy was computed before and after volume fluctuations only. Triangles were omitted from the summation if at least one of the triangle side lengths exceeded the cut-off distance, and an approximate tail correction was added (cf. supplemental information of [28]).

Simulations of liquid and gas phases were started from a dilute random configuration, simulations of solids from an fcc configuration. It is tacitly assumed that the spherical hydrogen molecules simulated in this work crystallize in an fcc lattice. The simulation ensembles for equilibrated for  $10^5$  cycles, with a cycle consisting of  $N$  attempted particle moves and—for  $NpT$  simulations—1 attempt to change the volume. The acceptance ratios for particle moves and volume fluctuations were both 50%. After equilibration,  $4 \times 10^5$  to  $6 \times 10^5$  cycles were performed, using 4–5 parallel threads, to obtain the thermodynamic averages.

### 2. Locating the triple point

During a Monte Carlo simulation the particles are displaced randomly according to

$$\mathbf{r}_i \leftarrow \mathbf{r}_i + \lambda \xi \mathbf{u}, \quad (56)$$

where  $\mathbf{r}_i$  denotes the location vector of particle  $i$ ,  $\mathbf{u}$  a unit vector with random direction,  $\xi$  a random number between 0 and 1, and  $\lambda$  the maximum displacement size. If the acceptance ratio  $a$  for displacements is kept constant by varying  $\lambda$  by means of a feedback loop, the average value of  $\lambda$  for this acceptance ratio,  $\lambda_a$  becomes a state property.

For this work, the melting pressure curves of classical hydrogen and neon were obtained with the entropy correlation method, which is based on the fact that, at high densities, the excess entropy is an almost linear function of  $\lambda_a^{-1}$  [29]. The latter is a byproduct of Monte Carlo simulations. By performing a series of  $NpT$  simulations over a sufficient pressure range it is possible to obtain differences of excess entropies, and ultimately differences of chemical potentials between the solid and the liquid phase. From these the phase transition point can be obtained. The procedure has been described in detail in Ref. 28.

Table III contains parts of the melting pressure curves of classical hydrogen and neon as well as the interpolated triple points.[30]

### 3. Computing the residual entropy

Once the triple points of classical hydrogen and neon were known, the excess chemical potentials and the excess entropies of the liquid phase could be obtained by thermodynamic integration. For this we performed

- a series of  $NpT$  simulations at a supercritical temperature  $T'$  (here: 80 K) up to 200 MPa,
- and a series of  $NVT$  simulations at  $\rho_L$  between  $T_{\text{trp}}$  and  $T'$ .

The excess chemical potential (i.e., the excess molar Gibbs energy) of the liquid at  $T = T_{\text{trp}}$  is then given by

$$\frac{\mu^r(\rho_L, T)}{RT} = \frac{1}{R} \int_T^{T'} \frac{U^r(\rho_L, T)}{T^2} dT + Z(\rho_L, T) - 1 + \int_0^{\rho_L} \frac{Z(\rho, T') - 1}{\rho} d\rho, \quad (57)$$

where  $Z(\rho, T) \equiv p/(\rho RT)$  is the compressibility factor. The integrands contain only entities that can be obtained from the computer simulations. The limiting value of the second integrand is

$$\lim_{\rho \rightarrow 0} \frac{Z(\rho, T')}{\rho} = B_2(T'), \quad (58)$$

TABLE III. Solid–liquid equilibrium of classical hydrogen and neon (temperature, pressure, liquid density, solid density), obtained with the entropy correlation method.

|              | $T/\text{K}$        | $p/\text{MPa}$ | $\rho^s/(\text{mol}/\text{dm}^3)$ | $\rho^l/(\text{mol}/\text{dm}^3)$ |
|--------------|---------------------|----------------|-----------------------------------|-----------------------------------|
| $\text{H}_2$ | 20.0                | −9.495         |                                   |                                   |
|              | 21.207 <sup>†</sup> | 0.000          | 54.39                             | 48.64                             |
|              | 22.0                | 6.197          | 54.73                             | 49.40                             |
|              | 24.0                | 19.935         | 55.52                             | 50.66                             |
|              | 26.0                | 33.348         | 56.20                             | 51.66                             |
| $\text{Ne}$  | 26.0                | −5.924         |                                   |                                   |
|              | 26.5                | −1.767         |                                   |                                   |
|              | 26.729 <sup>†</sup> | 0.000          | 74.63                             | 64.77                             |
|              | 27.0                | 1.988          | 74.64                             | 64.96                             |

†: indicates the approximate triple point

i.e., the 2nd virial coefficient. The integrals were constructed by constructing cubic spline functions through the integrand terms and performing the integrations analytically.

Finally, the excess entropy can be obtained from

$$S_m^{\text{ex}} = \frac{U_m^{\text{ex}} + \frac{p^{\text{ex}}}{\rho} - \mu^{\text{ex}}}{T} = \frac{U_m^{\text{ex}} - RT - \mu^{\text{ex}}}{T}. \quad (59)$$

### C. Neon data

The summary of the results for classical neon with two- and three-body effects yields:

- Triple-point temperature: 26.729 K
- Triple-point solid volume: 13.3987 cm<sup>3</sup>/mol
- Triple-point liquid volume: 15.4389 cm<sup>3</sup>/mol
- Triple-point liquid internal energy: -1837.54 J/mol
- Triple-point liquid excess chemical potential (same as excess Gibbs energy for a pure fluid): -1262.74 J/mol
- $\mathcal{L}$ : 0.255
- $s^+$ : 3.586

### D. Hydrogen data

The summary of the results for classical hydrogen with two- and three-body effects yields:

- Triple-point temperature: 21.21 K
- Triple-point solid volume: 18.3872 cm<sup>3</sup>/mol
- Triple-point liquid volume: 20.5585 cm<sup>3</sup>/mol
- Triple-point liquid internal energy: -1689 J/mol
- Triple-point liquid excess chemical potential (same as excess Gibbs energy for a pure fluid): -1212 J/mol
- $\mathcal{L}$ : 0.823
- $s^+$ : 3.705

## V. CRYOGEN TRENDS

Values of the shear viscosities and  $\tilde{\eta}$  were calculated with the default models in REFPROP 10.0 and presented in Fig. 8 for hydrogen and heavier species. The updated model for krypton [31] was also plotted, showing that it predicts viscosities more in line with those from the other heavy noble gases. While the shear viscosities in the liquid phase at the triple point differ by more than an order of magnitude ( $25\times$ ), the values of  $\tilde{\eta}$  differ within 10% of 4.35. Neon is above the heavy average of 4.35 by 4.6%. Its triple-point temperature has no uncertainty (is a fixed point of the ITS-90 temperature scale), while its density comes from the EOS, and there is significant scatter in the neon experimental data used to develop the viscosity model in NIST REFPROP. Whether neon *should* agree with the other heavier species is unclear.

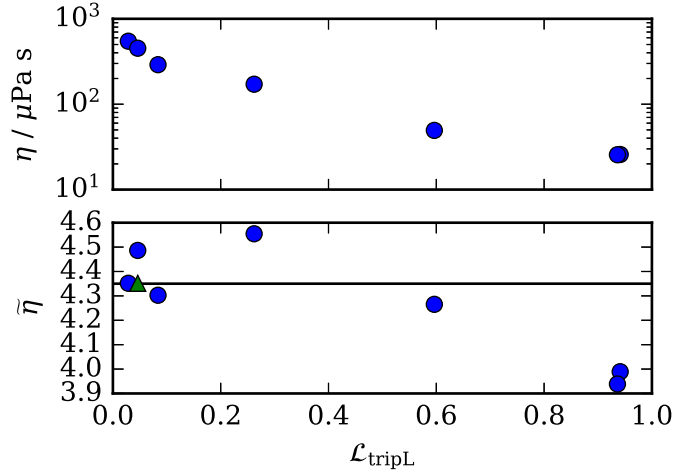

FIG. 8. Macroscopically scaled shear viscosities in the liquid phase at the triple point as a function of the length scale ratio  $\mathcal{L}$ . The value from the new model of Polychroniadou et al.[31] for krypton is indicated by a triangle.

## VI. THERMODYNAMIC MODELS FOR REAL GAS QUANTUM CORRECTION

### A. Boltzmann correction

Eq. 33.15 from Landau and Lifshitz[5], the correction to the total Helmholtz energy (given by  $F$ ) is

$$F = F_{\text{cl}} + \frac{\hbar^2}{24(k_{\text{B}}T)^2} \sum_i \frac{1}{m_i} \overline{\left(\frac{\partial U}{\partial q_i}\right)^2}_{q_j \neq i} \quad (60)$$

where if it is assumed that all the  $m_i$  are identical, it can instead be written as

$$\frac{F}{Nk_{\text{B}}} = \frac{F_{\text{cl}}}{Nk_{\text{B}}} + \frac{\hbar^2}{24(k_{\text{B}}T)^2 Nk_{\text{B}}m} \sum_i \overline{\left(\frac{\partial U}{\partial q_i}\right)^2}_{q_j \neq i} \quad (61)$$

which is equal to

$$\frac{F}{Nk_{\text{B}}} = \frac{F_{\text{cl}}}{Nk_{\text{B}}} + \frac{\hbar^2}{24(k_{\text{B}}T)^2 k_{\text{B}}m} \text{mean} \left( \overline{\left(\frac{\partial U}{\partial q_i}\right)^2}_{q_j \neq i} \right) \quad (62)$$

### B. Deiters quantum correction

In the approach from Deiters[32] the total molar Helmholtz energy  $a$  (residual + ideal-gas) is given in reduced form by

$$\alpha = a/(RT) \quad (63)$$

and it is given that

$$\alpha^{\text{quant}} = \alpha^{\text{cl}} + \Delta\alpha \quad (64)$$

The correction term is given in the form

$$\Delta\alpha = -3 \sum_{i=1}^{13} r_i y^i \quad (65)$$

with the coefficients  $r_i = [-4.9995174927\text{e-}1, -1.2867273248\text{e-}1, 2.6360453309\text{e-}2, -5.5253407160\text{e-}1, 2.2409938208\text{e+}0, -5.5702015921\text{e+}0, 8.6632912449\text{e+}0, -8.7278378272\text{e+}0, 5.7423465620\text{e+}0, -2.4445076274\text{e+}0, 6.4896811633\text{e-}1, -9.7758376489\text{e-}2, 6.3877188389\text{e-}3]$  for  $i = 1, 2, \dots$  with  $y = \lambda_{\text{th}}/L$ . This is plotted in Fig. 9

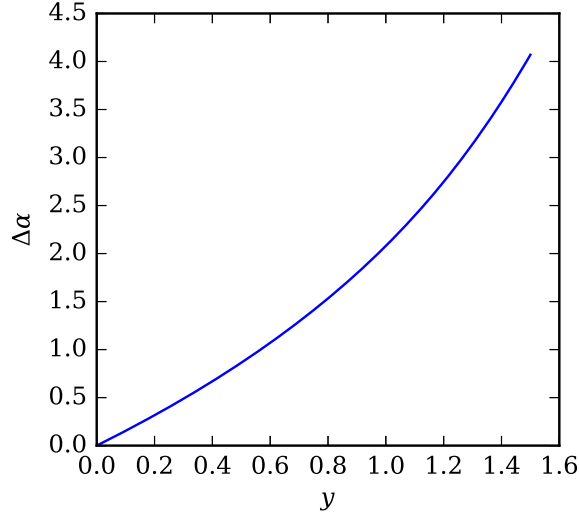

FIG. 9. Change in total reduced Helmholtz energy as a function of  $y$

The entropy is defined by

$$s = - \left( \frac{\partial a}{\partial T} \right)_{\rho_N} = -R \left( T \left( \frac{\partial \alpha}{\partial T} \right)_{\rho_N} + \alpha \right) \quad (66)$$

So given the linearity of the derivative operator applied to  $\alpha$ ,

$$\frac{\Delta s}{R} = - \left( T \left( \frac{\partial \Delta \alpha}{\partial T} \right)_{\rho_N} + \Delta \alpha \right) \quad (67)$$

in which  $\Delta s = s_{\text{quant}} - s_{\text{cl}}$ . The derivative of  $\Delta\alpha$  w.r.t.  $y$  is

$$\frac{d\Delta\alpha}{dy} = -3 \sum_{i=1}^{13} i r_i y^{i-1} \quad (68)$$

and that of  $y$  is equal to

$$T \left( \frac{\partial y}{\partial T} \right)_{\rho_N} = -y/2 \quad (69)$$

so the combined derivative term is

$$T \frac{d\Delta\alpha}{dT} = \frac{d\Delta\alpha}{dy} T \left( \frac{\partial y}{\partial T} \right)_{\rho_N} = -3 \sum_{i=1}^{13} (-i/2) r_i y^i \quad (70)$$

and the change in entropy is finally given by

$$\frac{\Delta s}{R} = - \left( T \left( \frac{\partial \Delta \alpha}{\partial T} \right)_{\rho_N} + \Delta \alpha \right) = 3 \sum_{i=1}^{13} (1 - i/2) r_i y^i \quad (71)$$

and is plotted in Fig. 10.

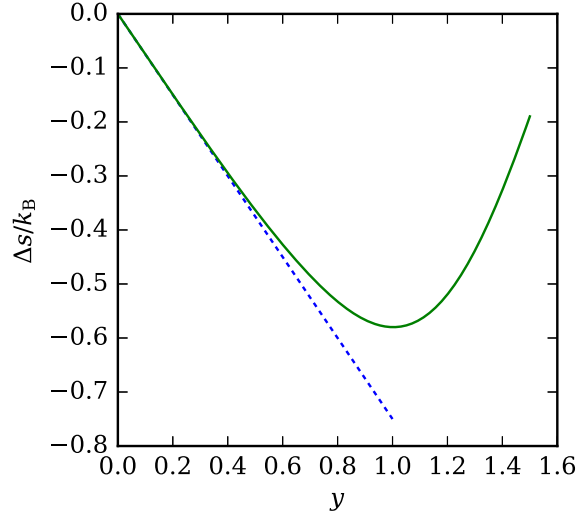

FIG. 10. Change in total reduced entropy as a function of  $y$ . Dashed curve shows the  $y^1$  term

The necessary Python code is:

```
r = [0, -4.9995174927e-1, -1.2867273248e-1, 2.6360453309e-2, -5.5253407160e-1,
2.2409938208e+0, -5.5702015921e+0, 8.6632912449e+0, -8.7278378272e+0,
5.7423465620e+0, -2.4445076274e+0, 6.4896811633e-1, -9.7758376489e-2,
6.3877188389e-3]
y = np.geomspace(1e-4, 1.5, 1000)
Deltaalpha = -3*sum([r[i]*y**i for i in range(1, 14)])
DeltaskB = 3*sum([(1-i/2)*r[i]*y**(i) for i in range(1, 14)])
```

### C. Hard sphere with quantum effects

In a virial expansion, the value of  $s^+$  is defined by [4, exercise 22-11]

$$s^+ = \sum_{n=1}^{\infty} \Theta_{n+1} \frac{\rho_N^n}{n} = \Theta_2 \rho_N + \Theta_3 \frac{\rho_N^2}{2} + \dots \quad (72)$$

with the derivative given by

$$\Theta_n = B_n + T \frac{dB_n}{dT}. \quad (73)$$

The quantity  $\Theta_2$  must be positive because the entropy must always be less than that of the non-interacting ideal gas at the same temperature and density. The ratio of  $\Theta_n$  to that of the classical fluid can help to explain the impact of quantum effects in dilute gases. If  $\Theta_n$  for the quantum fluid is greater than that of the classical fluid at the same temperature, the entropy decreases (or  $s^+$  increases) faster with density than the classical fluid.

The value of  $s^+$  is obtained from

$$s^+ = T \left( \frac{\partial \alpha^r}{\partial T} \right)_\rho + \alpha^r \quad (74)$$

The classical hard sphere, as a fully repulsive pair potential, has a one-dimensional phase diagram with the density (or packing fraction, or residual entropy, ...) as the independent variable. The addition of quantum effects adds a temperature dependence to the phase diagram. In the quantum-corrected hard sphere model, the relative de Broglie wavelength is defined by

$$\lambda^* = \frac{\lambda_{\text{th}}}{\sigma} = \frac{h}{\sigma \sqrt{2\pi m \varepsilon}} (T^*)^{-1/2} \quad (75)$$

and  $s^+$  can be expanded as

$$s^+ = \left( \frac{\partial \alpha^r}{\partial \lambda^*} \right)_y \left( T^* \frac{d\lambda^*}{dT^*} \right) + \alpha^r \quad (76)$$

with  $T^* d\lambda^*/dT^* = -\lambda^*/2$ .

Yoon and Scheraga[33] give the quantum-corrected second virial coefficient as a correction to the classical virial coefficient  $B_{\text{cl}}$ :

$$B_2 = B_{\text{cl}} k_0 \quad (77)$$

with

$$k_0 = 1 + a_1 \lambda^* + a_2 (\lambda^*)^2 + a_3 (\lambda^*)^3 \quad (78)$$

and  $a_1 = 1.08016$ ,  $a_2 = 0.752081$ , and  $a_3 = -0.489996$ . The value of  $\Theta_2$  is then obtained from

$$\Theta_2 = B_{\text{cl}} \left( k_0 + T^* \frac{dk_0}{dT^*} \right) = B_{\text{cl}} \left( k_0 + T^* \frac{d\lambda^*}{dT^*} \frac{dk_0}{d\lambda^*} \right) \quad (79)$$

or

$$\Theta_2 = B_{\text{cl}} \left( k_0 - \frac{\lambda^*}{2} \frac{dk_0}{d\lambda^*} \right) \quad (80)$$

with some intermediate calculations,

$$\frac{dk_0}{d\lambda^*} = a_1 + 2a_2 \lambda^* + 3a_3 (\lambda^*)^2 \quad (81)$$

$$\lambda^* \frac{dk_0}{d\lambda^*} = a_1 \lambda^* + 2a_2 (\lambda^*)^2 + 3a_3 (\lambda^*)^3 \quad (82)$$

the result is

$$\frac{\Theta_2}{\Theta_{2,cl}} = 1 + \frac{a_1}{2}\lambda^* - \frac{a_3}{2}(\lambda^*)^3 \quad (83)$$

With  $a_3$  being negative, the value of  $\frac{\Theta_2}{\Theta_{2,cl}}$  from this model is always positive. This means that quantum effects from this model consistently increase the value of  $\Theta_2$ .

The same general trend also holds at higher densities, as the calculated values in Fig. 11 indicate. The calculated values are obtained from the full EOS.

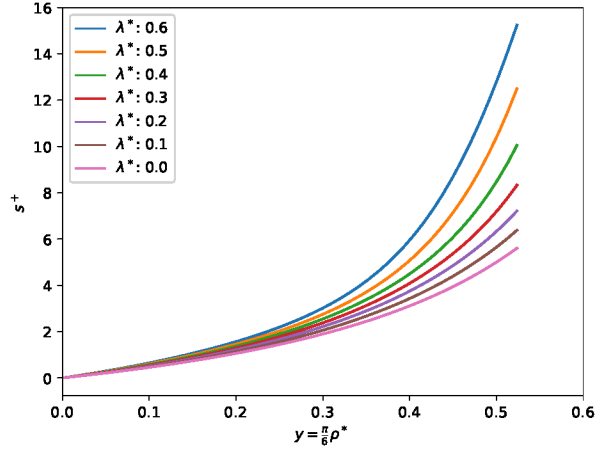

FIG. 11. Values of  $s^+$  for hard sphere with and without quantum effects

## VII. $s^+$ AT TRIPLE POINT

### A. Ideal-gas

The ideal-gas enthalpy is obtained from the integration (see for instance Ref. 2 or Ref. 34)

$$h = h_0^{(ig)} + \int_{T_{ref}}^T c_{p,0} dT \quad (84)$$

and the ideal gas internal energy ( $h^{(ig)} = u^{(ig)} + pv$ ) thus depends on

$$u^{(ig)} = h^{(ig)} - RT \quad (85)$$

since for an ideal gas,  $RT = pv$ . Thus,  $u^{(ig)}$  and  $h^{(ig)}$  do not depend on  $\rho$ , only  $T$ .

The entropy, on the other hand, has also density dependence, via

$$s^{(ig)} = s_0^{(ig)} + \int_{T_{ref}}^T \frac{c_{p,0}}{T} dT - R \ln \left( \frac{\rho T}{\rho_{ref} T_{ref}} \right) \quad (86)$$

which has the functional dependence  $s = f(T) - R \ln(\rho)$ , where  $f(T)$  collects all the temperature-dependent terms.

### B. Liquid phase

The change in entropy (all  $\Delta$  indicating liquid minus vapor) for phase change is equal to

$$\Delta s = (s^{ex} + s^{(ig)})_L - (s^{ex} + s^{(ig)})_V \approx s_L^{ex} - R \ln(\rho_L/\rho_V) \quad (87)$$

because the ideal-gas difference contributes a factor of  $(-R \ln(\rho_L) - (-R \ln(\rho_V)))$  at constant temperature and the value of  $s^+$  at the triple point in the liquid phase can be thus approximated by

$$s_{\text{tripL}}^+ \approx -\frac{\Delta h}{RT} - \ln\left(\frac{\rho_L}{\rho_V}\right) \quad (88)$$

where  $\Delta h$  is the enthalpy of vaporization. It is also to a good approximation given by  $\Delta u - RT$  because  $\Delta h = \Delta u + p\Delta v$ , and  $\Delta v$  is to an excellent approximation the negative of the vapor density, thus  $-pv/RT$  for the vapor phase is close to  $-1$  since the vapor phase at very low pressure is very ideal and  $Z = pv/(RT)$  is very close to 1.

The isothermal vaporization change in internal energy is given by

$$\Delta u = (u^{\text{ex}} + u^{(\text{ig})})_{\text{L}} - (u^{\text{ex}} + u^{(\text{ig})})_{\text{V}} \approx u_{\text{L}}^{\text{ex}} \quad (89)$$

since the ideal-gas terms are only temperature dependent (and thus their difference cancels) so with

$$\frac{\Delta h}{RT} = \frac{u_{\text{L}}^{\text{ex}}}{RT} - 1 \quad (90)$$

we have

$$s_{\text{tripL}}^+ \approx 1 - \frac{u_{\text{L}}^{\text{ex}}}{RT} - \ln\left(\frac{\rho_L}{\rho_V}\right) \quad (91)$$

Values of these terms and the overall term from the EOS are plotted in Fig. 12. The terms are shown relative to the values for argon. Neon has a smaller value of  $\ln(\rho_L/\rho_V)$  than argon, but its internal energy term is more in line with the other quantum-influenced cryogenics. Neither the internal energy nor the density ratio show a power-law deviation from the classical value that smoothly connects with the classical limit.

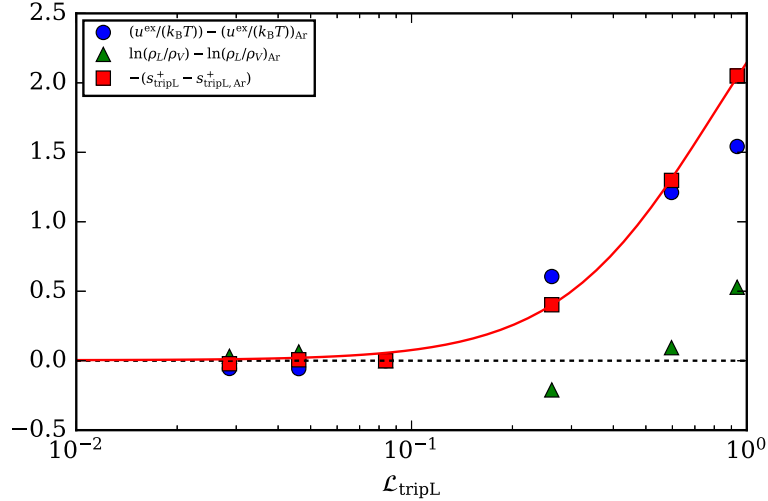

FIG. 12. Values at the triple point for the contributions that go into excess entropy for cryogenics, relative to the value for argon, as a function of the length-scale ratio  $\mathcal{L}$ . The solid curve is the correction term used in this work.

### C. Walker model

The values for the ab initio curves were digitized from Fig. 7 of Walker et al.[35], and the values of  $h/(\sigma\sqrt{m\epsilon})$  from Walker et al.[35] were divided by  $(2\pi)^{1/2}$  to yield the same definition of the de Broglie wavelength used in this work.

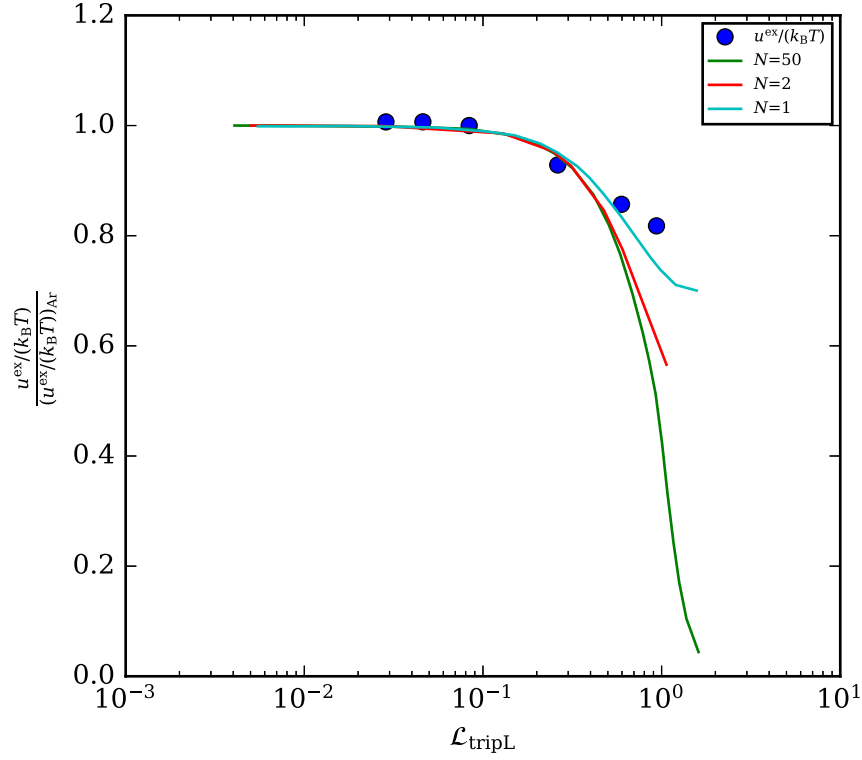

FIG. 13. Internal energy in the liquid phase at the SLV triple point relative to that of argon and the values of  $\epsilon/\epsilon(0)$  from Walker et al.[35] as a function of their number of terms in the Feynman-Hibbs summation ( $N$ ).

- 
- [1] I. H. Bell, U. K. Deiters, and A. M. M. Leal, *Ind. Eng. Chem. Res.* **61**, 6010 (2022).
  - [2] R. Span, *Multiparameter Equations of State - An Accurate Source of Thermodynamic Property Data* (Springer-Verlag, Berlin, 2000).
  - [3] L. E. Reichl, *A modern course in statistical physics* (Wiley, Weinheim, Germany, 1997), ISBN 9780471595205.
  - [4] T. L. Hill, *An Introduction to Statistical Thermodynamics* (Dover Publications, Inc., New York, 1986), ISBN 978-0486652429.
  - [5] L. D. Landau and E. M. Lifshitz, *Statistical physics, 2d rev. and enl. ed* (Pergamon Press, 1969), ISBN 0080091032.
  - [6] C. D. Muzny, M. L. Huber, and A. F. Kazakov, *J. Chem. Eng. Data* (2013).
  - [7] C. D. Muzny, M. L. Huber, and A. F. Kazakov, *J. Chem. Eng. Data* **67**, 2855 (2022).
  - [8] A. van Itterbeek and O. van Paemel, *Physica (Amsterdam)* **8**, 133 (1941).
  - [9] H. E. Johns, *Can. J. Res. A* **17**, 221 (1939).
  - [10] E. Kuss, *Z. Angew. Phys.* **4**, 203 (1952).
  - [11] A. Michels, A. Schipper, and W. Rintoul, *Physica (Amsterdam)* **19**, 1011 (1953).
  - [12] D. E. Diller, *J. Chem. Phys.* **42**, 2089 (1965).
  - [13] N. V. Tsederberg, V. N. Popov, and I. I. Andreev, *Teploenergetika* pp. 84–86 (1965).
  - [14] N. S. Rudenko and V. P. Slyusar, *Ukr. Fiz. Zh.* **13**, 917 (1968).
  - [15] F. A. Guevara, B. B. McInter, and D. Ottesen, *Phys. Fluids* **12**, 2493 (1969).
  - [16] V. N. Golubiev, *Zh. Prikl. Khim.* **43**, 706 (1970).
  - [17] H. Nabizadeh and F. Mayinger, *High Temp. - High Pressures* **31**, 601 (1999).
  - [18] S. Forster, *Cryogenics* **3**, 176 (1963).
  - [19] V. P. Slyusar, N. S. Rudenko, and V. M. Tret'yakov, *Ukr. Fiz. Zh.* **18**, 190 (1973).
  - [20] U. K. Deiters and R. J. Sadus, *J. Chem. Phys.* **150**, 134504:1 (2019).
  - [21] R. Hellmann, E. Bich, and E. Vogel, *Mol. Phys.* **106**, 133 (2008).
  - [22] K. Patkowski, W. Cencek, P. Jankowski, K. Szalewicz, J. B. Mehl, G. Garberoglio, and A. H. Harvey, *J. Chem. Phys.* **129**, 094304 (2008).
  - [23] B. M. Axilrod and E. Teller, *J. Chem. Phys.* **11**, 299 (1943).
  - [24] Y. Mutō, *J. Phys.-Math. Soc. Jpn. [Nihon Sūgaku Butsuri Gakkaishi]* **17**, 629 (1943), in Japanese.

- [25] R. Sadus and U. Deiters, J. Chem. Phys. (2023 (submitted)).
- [26] U. K. Deiters, *mc++* project homepage:  
<http://www.uni-koeln.de/deiters/mc++/index.html>.
- [27] U. K. Deiters, Z. Phys. Chem. **227**, 345 (2013).
- [28] U. K. Deiters and R. J. Sadus, J. Chem. Phys. **157**, 204504:1 (2022).
- [29] S. Yazdi Nezhad and U. K. Deiters, Mol. Phys. **115**, 1074 (2017).
- [30] Note1, more accurately: the states where the melting pressure is zero. However, the triple point pressures of these two substances are so small that their influence is negligible.
- [31] S. Polychroniadou, K. D. Antoniadis, M. J. Assael, and I. H. Bell, Int. J. Thermophys. **43**, 6 (2021).
- [32] U. K. Deiters, Fluid Phase Equilib. **10**, 173 (1983), ISSN 0378-3812, URL <https://www.sciencedirect.com/science/article/pii/0378381283800326>.
- [33] B. Yoon and H. A. Scheraga, J. Chem. Phys. **88**, 3923 (1988).
- [34] E. W. Lemmon, M. O. McLinden, and W. Wagner, J. Chem. Eng. Data **54**, 3141 (2009).
- [35] P. J. Walker, T. Zhao, A. J. Haslam, and G. Jackson, J. Chem. Phys. **156**, 154106 (2022).
